# Supplementary material for: Parametric correlations in energy density functionals
Source: arXiv:1910.13007 source file (2019-10-28)
Supplement: Supplementary file 1 [file suppl.pdf]

# Supplementary material.

TABLE I. Input data for fitting protocols of indicated CEDFs. The number $n_i$ of experimental (empirical) data points and adopted errors are presented for each type of data. These values are taken from Refs. [1–3]. In addition, employed empirical values for nuclear matter properties are shown.

| | NL5(E) | DDME-X | PCPK-X |
|---|---|---|---|
| 1 | 2 | 3 | 5 |
| 1. Masses $E$ (MeV) | | | |
| $n_1$ | 12 | 12 | 60 |
| $\Delta E$ [MeV] | $0.001E$ | $0.001E$ | 1.0 MeV |
| 2. Charge radii $r_{ch}$ (fm) | | | |
| $n_2$ | 9 | 9 | 17 |
| $\Delta r_{ch}$ [fm] | $0.002\,r_{ch}$ | $0.002\,r_{ch}$ | 0.02 |
| 3. Neutron skin $r_{skin}$ (fm) | | | |
| $n_3$ | N/A | 3 | N/A |
| $\Delta r_{skin}$ [fm] | $0.05\,r_{skin}$ | $0.05\,r_{skin}$ | N/A |
| 4. Nuclear matter properties | | | |
| $n_4$ | 4 | 4 | N/A |
| $E/A$ [MeV] | -16.0 | -16.0 | N/A |
| $\Delta E/A$ [MeV] | $0.05E/A$ | $0.05E/A$ | N/A |
| $\rho$ [fm$^-3$] | 0.153 | 0.153 | N/A |
| $\Delta\rho$ [fm$^-3$] | $0.1\rho$ | $0.1\rho$ | N/A |
| $K_0$ [MeV] | 250.0 | 250.0 | N/A |
| $\Delta K_0$ [MeV] | $0.025K_0$ | $0.1K_0$ | N/A |
| $J$ [MeV] | 33.0 | 33.0 | N/A |
| $\Delta J$ [MeV] | $0.1J$ | $0.1J$ | N/A |
| $N_{data}$ | 25 | 28 | 77 |
| $N_{par}$ | 6 | 8 | 9 |
| $N_{type}$ | 3 | 4 | 2 |

TABLE II. The parameters of the DD-ME2 and DDME-X functionals. Total penalty function $\chi^2_{total}$ and the contributions to it coming from nuclear matter properties ($\chi^2_{NM}$), binding energies ($\chi^2_E$), charge radii ($\chi^2_{Rch}$) and neutron skins ($\chi^2_{Nskin}$) are presented in the last part of the table. Note that these contributions are given both in absolute values and in percentages [in parentheses] with respect of $\chi^2_{total}$. The DD-ME2 parameters are taken from Ref. [2].

| | DD-ME2 | DDME-X |
|---|---|---|
| $m_\sigma$ | 550.123800 | 547.332728 |
| $g_\sigma$ | 10.539600 | 10.706722 |
| $g_\omega$ | 13.018900 | 13.338846 |
| $g_\rho$ | 3.683600 | 3.619020 |
| $b_s$ | 1.094300 | 1.334964 |
| $c_s$ | 1.705700 | 2.067122 |
| $c_o$ | 1.462000 | 1.605966 |
| $a_r$ | 0.564700 | 0.620220 |
| E/A | -16.140753 | -16.097256 |
| $\rho_0$ | 0.151930 | 0.151832 |
| $K_{inf}$ | 250.886065 | 267.046210 |
| $J_a$ | 32.899471 | 32.865829 |
| $L_0$ | 49.365384 | 47.806151 |
| $\chi^2_{total}$ | 39.24768 | 24.39452 |
| $\chi^2_{NM}$ (%) | 0.038 ( 0.1 %) | 0.4871 ( 2.0 %) |
| $\chi^2_E$ ((%) | 25.219 (64.3 %) | 16.1777 (66.3 %) |
| $\chi^2_{Rch}$ (%) | 12.459 (31.7 %) | 6.2067 (25.4 %) |
| $\chi^2_{Nskin}$(%) | 1.531( 3.9 %) | 1.523 ( 6.3 %) |

TABLE III. The same as Table II but for the parameters of the PC-PK1 and PC-X functionals. The PC-PK1 parameters are taken from Ref. [3].

| | PC-PK1 | PC-X |
|---|---|---|
| $\alpha_S$ | -0.39629D-03 | -0.40242D-03 |
| $\alpha_V$ | 0.26904D-03 | 0.27534D-03 |
| $\alpha_{TV}$ | 0.29502D-04 | 0.28188D-04 |
| $\beta_S$ | 0.86653D-10 | 0.85958D-10 |
| $\gamma_S$ | -0.38072D-16 | -0.37304D-16 |
| $\gamma_V$ | -0.36422D-17 | -0.49012D-17 |
| $\delta_S$ | -0.10911D-09 | 0.52181D-10 |
| $\delta_V$ | -0.43262D-09 | -0.59440D-09 |
| $\delta_{TV}$ | 0.41111D-09 | -0.52838D-09 |
| $\chi^2_{total}$ | 161.0056 | 93.1389 |
| $\chi^2_E$ | 149.5482 (92.9 % | 82.6613 (88.75 %) |
| $\chi^2_{Rch}$ (%) | 11.457 ( 7.1 %) | 10.4775 (11.25 %) |

There are the relations between some parameters of non-linear and point coupling models which are given

below according to Ref. [4].

$$\alpha_S = -\frac{g_\sigma^2}{m_\sigma^2}, \quad \delta_S = -\frac{g_\sigma^2}{m_\sigma^4},$$
$$\alpha_V = \frac{g_\omega^2}{m_\omega^2}, \quad \delta_V = \frac{g_\omega^2}{m_\omega^4}$$
$$\alpha_{TS} = \frac{g_\delta^2}{m_\delta^2}, \quad \delta_{TS} = \frac{g_\delta^2}{m_\delta^4}$$
$$\alpha_{TV} = \frac{g_\rho^2}{m_\rho^2}, \quad \delta_{TV} = \frac{g_\rho^2}{m_\rho^4} \quad (1)$$

Table IV compares numerical values of these parameters for three functionals. One can see that only $\alpha_S$ and $\alpha_V$ parameters defining the scalar and vector fields are similar in all functionals. On the contrary, there is a substantial difference between the $\delta_S$, $\delta_V$, $\alpha_{TV}$ and $\delta_{TV}$ parameters especially when comparing parameters extracted from NL5(E) and those in point coupling models.

TABLE IV. The comparison of selected parameters of point coupling CEDFs PC-PK1 and PC-X with those extracted from the NL5(E) [1] using Eqs. (1).

| Parameter | NL5(E) | PC-PK1 | PC-X |
|---|---|---|---|
| $\alpha_S$ | -0.41589D-03 | -0.39629D-03 | -0.40242D-03 |
| $\delta_S$ | -1.64182D-09 | -0.10911D-09 | 0.05218D-09 |
| $\alpha_V$ | 0.27702D-03 | 0.26904D-03 | 0.27534D-03 |
| $\delta_V$ | 0.45230D-09 | -0.43262D-09 | -0.59440D-09 |
| $\alpha_{TV}$ | 0.36074D-04 | 0.29502D-04 | 0.28188D-04 |
| $\delta_{TV}$ | 0.06196D-09 | 0.41111D-09 | -0.52838D-09 |

[1] S. E. Agbemava, A. V. Afanasjev, and A. Taninah, Phys. Rev. C **99**, 014318 (2019).
[2] G. A. Lalazissis, T. Nikšić, D. Vretenar, and P. Ring, Phys. Rev. C **71**, 024312 (2005).
[3] P. W. Zhao, Z. P. Li, J. M. Yao, and J. Meng, Phys. Rev. C **82**, 054319 (2010).
[4] T. Bürvenich, D. G. Madland, J. A. Maruhn, and P.-G. Reinhard, Phys. Rev. C **65**, 044308 (2002).
